# Supplementary material for: Relational Fusion Networks: Graph Convolutional Networks for Road Networks
Source: arXiv:2006.09030 source file (2020-09-14)
Supplement: Supplementary file 1 [file experiments_setup_to_appendix.tex]

\subsection{Data Set}
We extract the spatial representation of the Danish municipalities of Aalborg (AAL), Brønderslev (BRS), and Copenhagen (CPH) from \gls{osm}~\citep{osm}, and convert it to primal and dual graph representations as described in \cref{sec:road-network-modelling}.
\cref{tab:network-sizes} shows the sizes of the resulting graphs.

\begin{table}
  \centering
  \caption{Road network sizes.\label{tab:network-sizes}}
  \begin{tabular}{llll}
    \toprule
    & \emph{AAL} & \emph{BRS} & \emph{CPH} \\
    \midrule
    No.\ of Nodes ($|V|$) & $16\,294$ & $5\,889$ & $10\,738$ \\
    No.\ of Edges ($|E|$) & $35\,947$ & $13\,073$ & $26\,117$ \\
    No.\ of Between-Edges ($|B|$) & $94\,718$ & $34\,428$ & $72\,147$ \\
    \bottomrule
  \end{tabular}
\end{table}

We derive node attributes using a zone map from the Danish Business Authority\footnote{https://danishbusinessauthority.dk/plansystemdk}.
The map categorizes regions in Denmark as city zones, rural zones, and summer cottage zones. We use a node attribute for each zone category to indicate the category of an intersection.
In the \gls{osm} data, each road segment is categorized as one of nine road categories indicating their importance.
We use the road segment category and length as edge attributes.

As between-edge attributes, we use turn angles (between $0$ and $180$ degrees) relative to the driving direction between adjacent road segments as well as the turn directions, i.e., right-turn, left-turn, U-turn, or straight-ahead.
This separation of turn angle and turn direction resulted in superior results during early prototyping of our method.

\subsubsection{Attribute Encoding}
We encode each of the node attributes using a binary value, $0$ or $1$, thus obtaining node encodings with $3$ features per node.
Edge attributes are encoded as follows. Road categories are one-hot encoded, and road segment lengths are encoded as continuous values, yielding a total of $10$ features per edge.
We encode between-edge attributes by one-hot encoding the turn direction and representing the turn angle (between $0$ and $180$ degrees) using a continuous value, yielding an encoding with $5$ features per between-edge.

Conventional \glspl{gcn} can only use a single source of attributes.
The \glspl{gcn} we use in our experiments are therefore run on the dual graph and leverages the $10$ edge features.
However, to achieve more fair comparisons, we concatenate the source and target node features to the encodings of the edge attributes. This yields a final edge encoding with $16$ features per edge that we use throughout our experiments.
This allows the conventional \glspl{gcn} to also leverage node attributes.

Finally, we use min-max normalization s.t.\ all feature values are in the $[0; 1]$ range.
This normalization ensures that all features are on the same scale, thus making training with the gradient-based optimization algorithm we use in our experiments more stable.

\subsection{Experimental Setup}
We implement all algorithms based on neural networks using the MXNet\footnote{https://mxnet.incubator.apache.org/} deep learning library.
We make our implementation of the relational fusion networks publicly available online~\footnote{To be released upon acceptance.}.

\subsubsection{Hyperparameter Selection}
We use an architecture with two layers for all neural network algorithms.
For the \glspl{rfn}, we use $L_2$ normalization~\citep{graphsage} on some layers, i.e., $\textsc{Normalize}(\mathbf{h}) = \frac{\mathbf{h}}{|\mathbf{h}|_2}$ for a feature vector $\mathbf{h} \in \mathbb{R}^d$ where $|\cdot|_2$ is the $L_2$ norm, to ensure that the output of each layer is between $-1$ and $1$.
For driving speed estimation, we use $L_2$ normalization on the first layer. For speed limit classification, we found that training became more stable when using $L_2$ normalization on both layers.
In addition, we omit the $L_2$ normalization on the last layer of GraphSAGE for driving speed estimation; otherwise, the output cannot exceed a value of one.

We use the ReLU~\citep{relu} and softmax activation functions on the last layer for driving speed estimation and speed limit classification, respectively.
The ReLU function ensures outputs of the model are non-negative s.t.\ no model can estimate negative speeds.
Following the experimental setup of the authors of GraphSAGE~\citep{graphsage}, we use the ReLU activation function for the GraphSAGE pooling network.
For all attention coefficient networks in the GAT algorithm and relational fusion network, we use the LeakyReLU activation function with a negative input slope of $\alpha=0.2$, like the GAT authors~\citep{gat}.
For all other activation functions, we use the \gls{elu} activation function.
We select the remaining hyperparameters using a grid search and select the configuration with the best predictive performance on the validation set.

Based on preliminary experiments, we explore different learning rates $\lambda \in \{0.1, 0.01, 0.001\}$ in the grid search.
For GraphSAGE, GAT, and all RFN we explored $d \in \{32, 64, 128\}$ output dimensionalities of the first layer.
The MLP uses considerably fewer parameters than the other algorithms, and we therefore explore larger hidden layer sizes $d \in \{128, 256, 512\}$ for a fair comparison.

The GraphSAGE and GAT algorithms have additional hyperparameters.
GraphSAGE uses a pooling network to perform neighborhood aggregation. For each layer in GraphSAGE, we set the output dimension of the pooling network to be double the output dimension of the layer in accordance with the authors' experiments~\citep{graphsage}.

The GAT algorithm uses multiple attention heads that each output $d$ features at the first hidden layer.
These features are subsequently concatenated yielding an output dimensionality $h \cdot d$, where $h$ is the number of attention heads.
Based on the work of the authors~\citep{gat}, we explore different values of $h \in \{1, 2, 4, 8\}$ during the grid search.
However, due to the concatenation, large values of $h$ combined with large values of $d$ make the GAT network very time-consuming to train.
We therefore budget these parameters s.t.\ $h \cdot d \leq 256$ corresponding to, e.g., a GAT network with $64$ output units from $4$ attention heads.

\subsubsection{Model Training and Evaluation}\label{sec:model-training}
We initialize the neural network weights using Xavier initialization~\citep{xavier} and train the models using the ADAM optimizer~\citep{adam} in batches of $256$ segments.
In preliminary experiments, we observed that all models converged within $20$ and $30$ epochs for driving speed estimation and speed limit classification, respectively.
We therefore use these values for training.

A number of algorithms for efficient training of \glspl{gcn} have been proposed in the literature~\citep{graphsage,fastgcn, vrgcn, asgcn, layer-dependent-sampling}. To the best of our knowledge, \glspl{rfn} are compatible with all of them.
For the purposes of these experiments, we use a mini-batch training approach similar to that of \citet{graphsage}, where the \glspl{gcn} are trained on a sub-network induced by each batch s.t.\ the graph convolutional models only perform the computationally expensive graph convolutions on the relevant parts of the network.
However, to avoid the computational overhead of generating the sub-network for each batch in each epoch, we pre-compute the batches and shuffle the batches during each epoch.
In order to ensure that the mini-batches provide good approximations of the global gradient, we compute the batches in a stratified manner.
In the case of the driving speed estimation task, we select road segments for each batch s.t.\ the distribution of road categories in the batch is similar to the distribution of the entire training set.

\paragraph{Driving Speed Estimation}
In this experiment, we aim to estimate the mean driving speed on each road segment in a road network.
For the driving speed estimation task we evaluate each model by measuring the \gls{mae} between the mean recorded speed of a segment and the model output.
Let $D=\bigcup_{i=1}^{N}\{(s_i, Y_i)\}$ be a dataset, e.g., the training set, where $(s_i, Y_i)$ is a unique entry for road segment $s_i \in E$ and $Y_i = {y_{i, 1}, \dots, y_{i, j} }$ is a set of recorded speeds on road segment $s_i$.
Formally, we measure the error of each model as $\text{MAE} = \frac{1}{N}\sum_{(s, Y) \in D} |\hat{y} - \bar{Y}|$ where $\hat{y}$ is the estimated driving speed of segment $s$ of the model and $\bar{Y}=\sum_{y \in Y} \frac{y}{|Y|}$ is the mean recorded speed for a segment $s$.
$\bar{Y_i}$ is not representative of the population mean of a road segment $s_i$ if it contains very few speed records.
We therefore remove entries $(s_i, Y_i)$ from $D$ if there are fewer than ten recorded speeds in $Y_i$ when measuring \gls{mae}.

The recorded driving speeds are heavily concentrated on a few popular road segments.
We therefore weigh the contribution of each recorded speed to the loss s.t.\ each road segment contribute evenly to the loss independent of their frequency in the dataset.
Formally, we minimize the average (over segments) \gls{mse} loss of a model: $\textsc{AMSE-Loss} = \frac{1}{N}\sum_{(s, Y) \in D} \sum_{y \in Y} \frac{(\hat{y} - y)^2}{|Y|}$ where $\hat{y}$ is the estimated driving speed of segment $s$ of the model.

\paragraph{Speed Limit Classification}
We follow the methodology of \citet{workshop} and use random over-sampling with replacement when training the model to address the large imbalance in speed limit frequencies.
This ensures that all speed limits occur with equal frequency during training.
We train the model to minimize the categorical cross entropy on the over-sampled training set and measure model performance using the macro $F_1$ score which punishes poor performance equally on all speed limits, irrespective of their frequency.

During training, we found that all algorithms were prone to overfitting on the training set.
In addition, the model decision boundaries between speed limits are very sensitive during training causing the macro $F_1$ score on the validation set to be highly unstable.
We therefore use a variant of early stopping to regularize the model: we store the model after each training epoch and select the version of the model with the highest macro $F_1$ on the validation set.
Finally, we restore this model version for final evaluation on the test set.
